# Supplementary material for: Competing Models
Source: arXiv:1907.03809 source file (2021-11-11)
Supplement: Supplementary file 1 [file KnownPappendix.tex]

\paragraph{Known Variance.}
%What happens when the variance $\seps$ of the noise-term $\epsilon$ is commonly known among the agents? This is an extreme special case of our model; it may be realistic in some situations, but not in others.\footnote{Indeed, this assumption may be problematic in some environments. When variance is known, agents with incorrect models of the world will, as data accrues, observe that their model has an empirical error different (higher) than the known $\sigma^2$, because the model disregards some covariates relevant for prediction.  For $n$ large, this disparity in the empirical error and the (known) $\sigma^2$ should lead them to question their underlying model. However, as is standard with Bayesians with dogmatic beliefs (here they have degenerate beliefs on $\sigma^2$) they do not. When the dataset is not too large, however, such issues will not arise.}

\begin{restatable}{proposition}{knownvariance}\label{prop:knownvariance}
Suppose agents have Normal priors on $\beta$ with shared hyper-parameter $\gamma$, but their prior on $\epsilon$ is degenerate at $\seps$. Suppose that all agents believe the joint distribution of the covariates, $P$, is such that $\mathbb{E}_P[xx'] = \mathbb{I}_k$. Fix a prior $\pi'$ with $J(\pi')= J'$. For any number $k'$ smaller than $|J'|$, and any dataset $D_n$ for $n >0$, there exists a prior $\pi$ such that $J(\pi)\equiv J \subseteq J'$ with $|J|=k'$ and such that $L^*(\pi, D_n) < L^*(\pi', D_n).$
\end{restatable}

\begin{proof}
Suppose the known variance of $\epsilon$ is $\seps$. Then for any agent with prior $\pi$, upon seeing data $D_n$, the posterior expected loss evaluates to:
\begin{align*}
    L^*(\pi_j, D_n) = \seps + \trace(\mathbb{V}_{\pi}[\beta|D_n]),
\end{align*}
where we have assumed that $\mathbb{E}_{P}[xx']=\mathbb{I}_k$.  From the formula for posterior variance of $\beta$ for agents with this prior (recall \eqref{equation:PosterVariance}), we have that $\mathbb{V}_{\pi}[\beta|D_n] = \seps (X'_J X_J + \gamma |J| \mathbb{I}_{|J|})^{-1}$. 

Without loss of generality, suppose the larger model $J'$ is the entire set of covariates of size $k$. We need to show that there exists a model $J$ of size $|J|<k$ such that 
\begin{align*}
    \trace (X'X + \gamma k \mathbb{I}_k)^{-1} \geq \trace (X'_J X_J + \gamma |J| \mathbb{I}_{|J|})^{-1}.
\end{align*}
In particular let $J$ be such that $\sum_{j\in J} e'_j (X'X + \gamma k \mathbb{I}_{k})^{-1} e_j \leq \sum_{j\in J''} e'_j (X'X + \gamma k \mathbb{I}_{k})^{-1} e_j $ for any $J''$ such that $|J''| = |J|$. Here $e_j$ is the $j^{\text{th}}$ column of the $k \times k $ identity matrix.
Then, it must be the case that
\begin{align*}
    \trace (X'X + \gamma k \mathbb{I}_k)^{-1} \geq \frac{k}{|J|} \sum_{j\in J} e'_j (X'X + \gamma k \mathbb{I}_{k})^{-1} e_j.
\end{align*}
Therefore it is sufficient to show that for this model $J$, we have
\begin{align*}
    \frac{k}{|J|} \sum_{j\in J} e'_j (X'X + \gamma k \mathbb{I}_{k})^{-1} e_j \geq \trace (X'_J X_J + \gamma |J| \mathbb{I}_{|J|})^{-1}.
\end{align*}
Without loss we can renumber the indices so that $J = \{1,2, \ldots, |J|\}$. Let $L$ denote the set of remaining indices, i.e. $L = \{|J|+1, \ldots , k\}$. We can thus write the left hand size of the inequality as:
\begin{align*}
    &\frac{k}{|J|} \sum_{j\in J} e'_j \left(\begin{array}{cc}
        X_J'X_J + \gamma k \mathbb{I}_{|J|} & X_J' X_L \\
        X_L' X_J & X_L' X_L + \gamma k \mathbb{I}_{|L|}
    \end{array}\right)^{-1} e_j.
    \intertext{Using the standard formula for block inverse of a matrix we can write this as:}
    =& \frac{k}{|J|} \sum_{j\in J} e'_j \left(\begin{array}{cc}
        A_1 & A_2 \\
        A_3 & A_4
    \end{array}\right) e_j.
    \intertext{where $A_1 = (X_J'X_J + \gamma k \mathbb{I}_{|J|} - X_J' X_L (X_L' X_L + \gamma k \mathbb{I}_{|L|})^{-1} X_L' X_J)^{-1}$. Substituting in we have}
    =& \frac{k}{|J|} \trace (X_J'X_J + \gamma k \mathbb{I}_{|J|} - X_J' X_L (X_L' X_L + \gamma k \mathbb{I}_{|L|})^{-1} X_L' X_J)^{-1}.
\end{align*}
Therefore, taking $\frac{k}{|J|}$ to the other side, we are left to show that 
\begin{align}\label{eqn:ineq3}
\trace (X_J'X_J + \gamma k \mathbb{I}_{|J|} - X_J' X_L (X_L' X_L + \gamma k \mathbb{I}_{|L|})^{-1} X_L' X_J)^{-1} \geq \trace (\frac{k}{|J|} X_J'X_J + \gamma k \mathbb{I}_{|J|})^{-1}.
\end{align}
Next, given 4 matrices A,B,C, and D where $A$ and $C$ are invertible, by the Woodbury matrix identity (see e.g. equation (0.7.4.1) of \cite{horn1990matrix}),
\begin{align*}
    (A + BCD)^{-1} &= A^{-1} - A^{-1} B (C^{-1}+ D A^{-1} B) D A^{-1}.
\intertext{Suppose we define}
A  &= X_J'X_J + \gamma k \mathbb{I}_{|J|},\\
B &= - X_J' X_L,\\
C &= (X_L' X_L + \gamma k \mathbb{I}_{|L|})^{-1} ,\\
D&= X_L' X_J. 
\end{align*}
Note that in this case, $A$ and $C$ are invertible by observation. In light of this, and the linearity of the Trace operator, we can rewrite the left hand side of \eqref{eqn:ineq3} as
\begin{align*}
    & \trace (A^{-1} - A^{-1} B (C^{-1}+ D A^{-1} B) D A^{-1}),\\
    =& \trace A^{-1} - \trace (A^{-1} B (C^{-1}+ D A^{-1} B) D A^{-1}),\\
    =& \trace(X_J'X_J + \gamma k \mathbb{I}_{|J|})^{-1} - \trace (A^{-1} B (C^{-1}+ D A^{-1} B) D A^{-1}),
\end{align*}
where $A,B,C$ and $D$ are as defined above. So \eqref{eqn:ineq3} can be written as:
\begin{align*}
   \trace(X_J'X_J + \gamma k \mathbb{I}_{|J|})^{-1} - \trace (A^{-1} B (C^{-1}+ D A^{-1} B) D A^{-1}) \geq  \trace (\frac{k}{|J|} X_J'X_J + \gamma k \mathbb{I}_{|J|})^{-1}.
\end{align*}
To show this inequality it is therefore sufficient to show that
\begin{align}
  & \trace (A^{-1} B (C^{-1}+ D A^{-1} B) D A^{-1}) \leq 0,\label{eqn:reqineq4} \\
   & \trace(X_J'X_J + \gamma k \mathbb{I}_{|J|})^{-1} \geq \trace (\frac{k}{|J|} X_J'X_J + \gamma k \mathbb{I}_k)^{-1}.\label{eqn:reqineq5}
\end{align}
We now show each of these in turn. Let us start with the first. Note that $B = -D'$ we have:
\begin{align*}
    \eqref{eqn:reqineq4} \iff &\trace (A^{-1} D' (C^{-1}- D A^{-1} D') D A^{-1}) \geq 0.
    \intertext{In turn, since $A$ is symmetric, so is $A^{-1}$, so defining $Q \equiv A^{-1}D'$}
    \iff &\trace (Q (C^{-1}- D A^{-1} D') Q') \geq 0.
\end{align*}
Since $Q M Q'$ is a positive semidefinite matrix if $M$ is a positive semidefinite matrix (see e.g. Observation 7.1.8 of \cite{horn1990matrix}), it is sufficient to show that $(C^{-1}- D A^{-1} D')$ is a positive semidefinite matrix (the trace of a matrix equals the sum of all its eigenvalues, and the eigenvalues of a positive semidefinite matrix are all non-negative). So to show \eqref{eqn:reqineq4}, it is sufficient to show that $(C^{-1}- D A^{-1} D')$ is positive semidefinite. To see this, observe that:
\begin{align*}
   &(C^{-1}- D A^{-1} D'),\\
   =& X_L'X_L + \gamma k \mathbb{I}_{|L|} - X_L' X_J (X_J' X_J +\gamma k \mathbb{I}_{|J|})^{-1} X_J' X_L,\\
   =& X_L' \left( \mathbb{I}_{N} - X_J (X_J' X_J +\gamma k \mathbb{I}_{|J|})^{-1} X_J'\right) X_L +  \gamma k \mathbb{I}_{|L|}.
\end{align*}
It is therefore sufficient to show that each of these two matrices are positive semidefinite. The latter is positive definite by observation. To show that the former is positive semidefinite, by another appeal to Observation 7.1.8 of \cite{horn1990matrix}, it is sufficient to show that $\left( \mathbb{I}_{k} - X_J (X_J' X_J +\gamma k \mathbb{I}_{|J|})^{-1} X_J'\right)$ is positive semidefinite. But observe that:
\begin{align}
&\mathbb{I}_{k} - X_J (X_J' X_J +\gamma k \mathbb{I}_{|J|})^{-1} X_J', \nonumber\\
=& \mathbb{I}_{k} -\frac{1}{\gamma k} X_J (\frac{1}{\gamma k} X_J' X_J + \mathbb{I}_{|J|})^{-1} X_J' \label{term1}.
\end{align}
Now, we know that for any square matrix $P$, 
\begin{align*}
(\mathbb{I} + P)^{-1} &= I - (\mathbb{I} + P)^{-1} P,\\
&= I - P + (\mathbb{I} + P)^{-1} P^2,\\
&= I + \sum_{j=1}^{\infty} (-1)^j P^j. 
\end{align*}
Substituting in $P = \frac{1}{\gamma k} X_J'X_J$, we have that
\begin{align*}
X_J (\frac{1}{\gamma k} X_J' X_J + \mathbb{I}_{|J|})^{-1} X_J' &= X_J \left(\mathbb{I}_{|J|} - \sum_{j=1}^\infty (-\frac{1}{\gamma k})^j (X_J'X_J)^j \right)X_J',\\
&= X_J X_{J}' - \sum_{j=1}^\infty (-\frac{1}{\gamma k})^j (X_JX_J')^{j+1},\\
&= (X_J X_J') (\mathbb{I}_{|J|} - \sum_{j=1}^\infty (-\frac{1}{\gamma k})^j (X_JX_J')^{j}),\\
&= (X_J X_J') (\mathbb{I}_{|J|} + \frac{1}{\gamma k} X_J X_J')^{-1}.
\end{align*}
Therefore we have that
\begin{align*}
\eqref{term1} &= \mathbb{I}_{k} -\frac{1}{\gamma k} (X_J X_J') (\mathbb{I}_{|J|} + \frac{1}{\gamma k} X_J X_J')^{-1},\\
&= \mathbb{I}_{k} - (X_J X_J') (\gamma k\mathbb{I}_{|J|} +  X_J X_J')^{-1},\\
&= \gamma k (\gamma k\mathbb{I}_{|J|} +  X_J X_J')^{-1}.
\end{align*}
which is positive definite by observation. 

We are left, then, to show \eqref{eqn:reqineq5}, i.e. that:
\begin{align*}
     & \trace(X_J'X_J + \gamma k \mathbb{I}_{|J|})^{-1} \geq \trace (\frac{k}{|J|} X_J'X_J + \gamma k \mathbb{I}_k)^{-1},\\
\iff& \trace ((X_J'X_J + \gamma k \mathbb{I}_{|J|})^{-1} -  (\frac{k}{|J|} X_J'X_J + \gamma k \mathbb{I}_k)^{-1}) \geq 0.
\end{align*}
Algebra shows
\begin{align*}
    &\trace((X_J'X_J + \gamma k \mathbb{I}_{|J|})^{-1} -  (\frac{k}{|J|} X_J'X_J + \gamma k \mathbb{I}_k)^{-1}),\\
=& \trace ((X_J'X_J + \gamma k \mathbb{I}_{|J|})^{-1} \left(\frac{k-|J|}{|J|} X_J'X_J \right) (\frac{k}{|J|} X_J'X_J + \gamma k \mathbb{I}_k)^{-1}),\\
=&\trace ( \frac{k-|J|}{|J|} X_J (X_J'X_J + \gamma k \mathbb{I}_{|J|})^{-1} (\frac{k}{|J|} X_J'X_J + \gamma k \mathbb{I}_k)^{-1} X_J' ).
\end{align*}
The final matrix into the trace operator is positive semidefinite by Observation 7.1.8 of \cite{horn1990matrix}.
\end{proof}

\begin{restatable}{proposition}{beforedata}
\label{prop:beforedata}
Suppose agents have Normal Inverse-Gamma priors with shared hyper-parameters $( a_0,b_0, \gamma)$. Suppose further that $x \sim \mathcal{N}_{k}(0, \mathbb{I}_k)$ independently of $\epsilon$.  Fix a prior $\pi$. For any prior $\pi'$, such that $|J(\pi')|< |J(\pi)|$,  when $\gamma \rightarrow 0$ we have that
$$\mathbb{E}_{m(\pi')} [L^* (\pi', D_n) ] < \mathbb{E}_{m(\pi)} [L^*(\pi,D_n)],$$
whenever $n > |J(\pi)|+1$. Here the outer expectation is taken over the agents' `marginal' distribution of the data $m(\pi) : = \int q_{\theta}(D_n) \pi(\theta) d \theta$.\footnote{Hence, the expression $\mathbb{E}_{m(\pi')} [L^* (\pi', D_n) ]$ is the \emph{Bayes risk} of the \emph{Bayes Predictor}. See Equation 1.14 in Chapter 1.6 in \cite{Ferguson67}.}  
\end{restatable}

\begin{proof}
For an agent with prior $\pi$ the agent's ex-ante expected loss on seeing a dataset of size $n$ is
\begin{align*}
\mathbb{E}_{m(\pi)}[L^{*}(\pi,D_n)] &= \int_{\theta= (\beta,\seps)} \int_{D_n} \int_{y,x} (y- x'\widehat{\beta}(D_n) )^2 dQ_{\theta}(y,x) dQ_{\theta} (D_n) d \pi (\theta).
\intertext{The agents' statistical model is  $y=x' \beta  + \epsilon$, $\epsilon\sim\mathcal{N}(0,\seps)$}
&= \int_{\theta= (\beta,\seps)} \int_{D_n} \int_{y,x} (x' \beta  +\epsilon-x' \widehat{\beta}(D_n) )^2 dQ_{\theta}(x,\epsilon) dQ_{\theta} (D_n) d \pi (\theta),\\
&= \int_{\theta= (\beta,\seps)} \int_{D_n} \int_{x,\epsilon} ((x'(\beta -\widehat{\beta}(D_n)) )^2 + \epsilon^2) dQ_{\theta}(x,\epsilon) dQ_{\theta} (D_n) d \pi (\theta),\\
&= \mathbb{E}_{\pi}[\seps] + \int_{\theta= (\beta,\seps)} \int_{D_n} \int_{x} (x'(\beta -\widehat{\beta}(D_n)) )^2  dQ_{\theta}(x) dQ_{\theta} (D_n) d \pi (\theta),\\
&=  \mathbb{E}_{\pi}[\seps] + \int_{\theta= (\beta,\seps)} \int_{D_n} \left(\int_{x} ((\beta -\widehat{\beta}(D_n))' x x' (\beta -\widehat{\beta}(D_n))  dQ_{\theta}(x)\right) dQ_{\theta} (D_n) d \pi (\theta),\\
&= \mathbb{E}_{\pi}[\seps] + \int_{\theta= (\beta,\seps)} \int_{D_n}  ((\beta -\widehat{\beta}(D_n))' (\beta -\widehat{\beta}(D_n))  dQ_{\theta} (D_n) d \pi (\theta).
\end{align*}
Where the last equality follows since $\mathbb{E}_{P}[xx']= \mathbb{I}$ by assumption. 
Now, since $\gamma  \rightarrow 0$ by assumption, for dataset $D_n = (Y, X)$, we have that $\widehat{\beta}(D_n) = (X_{J(\pi)}'X_{J(\pi)})^{-1}X_{J(\pi)}' Y$. In a slight abuse of notation abbreviate $J(\pi)$ as $J$.  Every agent is calculating expectations using their \emph{own} statistical model. Consequently, if the agent's statistical model uses the covariates in the set $J$, and $(Y,X_J) \sim Q_{\theta}$, then from the agent's perspective 
\begin{align*}
    (\widehat{\beta}(D_n)-\beta )
    &= (X_J'X_J)^{-1} X_J' e,
\end{align*}
    where $e$ is the $n \times 1$ vector collecting the normally distributed errors $\epsilon_i$. 
Substituting back in we have that:
\begin{align*}
    \mathbb{E}_{m(\pi)}[L^{*}(\pi,D_n)] &=  \mathbb{E}_{\pi}[\seps] + \int_{\theta= (\beta,\seps)} \int_{D_n}  ((\beta -\widehat{\beta}(D_n))' (\beta -\widehat{\beta}(D_n))  dQ_{\theta} (D_n) d \pi (\theta),\\
    &= \mathbb{E}_{\pi_J}[\seps] + \int_{\theta= (\beta,\seps)} \int_{D_n}  \left(e' X_J  (X_J'X_J)^{-1} (X_J'X_J)^{-1} X_J' e\right) dQ_{\theta} (D_n) d \pi (\theta),\\
    \intertext{and since $e' X_J  (X_J'X_J)^{-1} (X_J'X_J)^{-1} X_J' e$ is a scalar}
     &= \mathbb{E}_{\pi}[\seps] + \int_{\theta= (\beta,\seps)} \int_{D_n}  \trace(e' X_J  (X_J'X_J)^{-1} (X_J'X_J)^{-1} X_J' e) dQ_{\theta} (D_n) d \pi_J (\theta).\\
     \intertext{Using the cyclic property of the trace operator,}
        &= \mathbb{E}_{\pi}[\seps] + \int_{\theta= (\beta,\seps)} \int_{D_n}  \trace((X_J'X_J)^{-1} X_J' ee' X_J  (X_J'X_J)^{-1} ) dQ_{\theta} (D_n) d \pi (\theta).\\
    \intertext{By assumption, $X_J$ and $e$ are independent and $\mathbb{E}_{Q_{\theta}}[ee'] = \seps \mathbb{I}_n$ for all $\theta$ in the support of $\pi$. Thus,}
    &=\mathbb{E}_{\pi}[\seps] + \int_{\theta= (\beta,\seps)} \seps \int_{X_J} \trace ((X_J'X_J)^{-1} X_J' X_J  (X_J'X_J)^{-1})  dQ_{\theta} (X_J) d \pi_J (\theta),\\
     &=\mathbb{E}_{\pi}[\seps] + \int_{\theta= (\beta,\seps)} \seps \int_{X_J}\trace  (X_J'X_J)^{-1}  dQ_{\theta} (X_J) d \pi_J (\theta),\\
     &= \mathbb{E}_{\pi}[\seps] \left( 1+ \frac{|J|}{n-|J|-1}\right).
\end{align*}
The last equation follows because when $x\sim\mathcal{N}(0,\mathbb{I}_{k})$, $(X_J' X_J)$ is a Wishart distribution $\mathcal{W}(\mathbb{I}_J, n)$. Thus, $(X_J' X_J)^{-1}$ has an inverse Wishart distribution and its expectation equals $\mathbb{I}_{J}/(n-|J|-1)$,
provided $n>|J|+1$. Finally
\[ \frac{J'}{n-J'-1} < \frac{J}{n-J-1}, \]
if and only if $n>1$. Since $\mathbb{E}_{\pi}[\seps]$ is common across all agents by assumption, the result follows.
\end{proof}

\begin{restatable}{proposition}{onedata} 
\label{prop:1data} 
Suppose all agents have Normal-Inverse Gamma priors with shared hyper-parameters $(a_0,b_0, \gamma)$. Suppose that all agents believe the joint distribution of the covariates, $P$, is such that $\mathbb{E}_P[xx'] = \mathbb{I}_k$. Suppose that for every single covariate model, i.e. every $J$ such that $|J|=1$, there is an agent with that model and that all agents use at least one covariate. If these agents compete after seeing a dataset which consists of a single observation, i.e., $n=1$, then the winner is always one of these agents with a single variable model, regardless of which other models are represented.
\end{restatable}

\begin{proof}
Denote the single datapoint as $D_1 = (Y,X)$, where $Y \in \mathbb{R}$ and $X \in \mathbb{R}^{1 \times k}$ ($k$ is the number of covariates), and $X=x'$. First, observe that for any agent $j$ with a single explanatory variable $\kappa$ in his model (denoted $x_{\kappa}$). By Lemma \ref{lemma:postlossNormalInverseGamma}
\begin{align*}
L^*(\pi_j, D_1) &= \frac{b_0 + \frac12 \left(y^2 - \frac{y^2x_{\kappa}^2}{x_{\kappa}^2 + \gamma}\right) }{a_0 - \frac12} \left(1 + \frac{1}{x_{\kappa}^2 + \gamma}\right), \\
&= \frac{b_0 + \frac12  \frac{y^2\gamma}{x_{\kappa}^2 + \gamma} }{a_0 - \frac12} \left(1 + \frac{1}{x_{\kappa}^2 + \gamma}\right).
\end{align*}
The winning agent among the single variable models will therefore clearly be the agent with the variable $\kappa$ that maximizes $x_{\kappa}$. Without loss of generality, call this variable $1$.

To economize on notation, now consider the full model with all the explanatory variables, it will be clear from the logic that this argument will work for any model larger than a single variable. For an agent $j$ with all $k$ variables, we know that 
\begin{align*}
L^*(\pi_j, D_1) = \frac{b_0 + \frac{y^2}{2} \left(1- X(X'X + \gamma k \mathbb{I}_k )^{-1} X'\right)}{a_0 - \frac12} \left(1 + \mathrm{tr}\left[\left(X'X + \gamma k \mathbb{I}_k\right)^{-1}\right] \right).
\end{align*}
To show that this model always loses, we need to show that this model's loss is always larger than the ``best'' single variable model. To do this, it is sufficient to show that: 
\begin{align*}
&(1- X(X'X + \gamma k \mathbb{I}_k)^{-1}X') \geq \frac{\gamma}{x_1^2 + \gamma},\\
& \mathrm{tr}\left[\left(X'X + \gamma k \mathbb{I}_k\right)^{-1}\right] \geq \frac{1}{x_1^2 + \gamma}. 
\end{align*}
We will handle each of these separately. Let's start with the second. It is well known that for any positive definite symmetric matrix $A$ the $j$-th diagonal element of its inverse is larger than the reciprocal of its $j$-th diagonal element. That is,
\[(A^{-1})_{jj} \geq (A_{jj})^{-1}.\]
Consequently, 
\begin{eqnarray*}
\textup{tr} \left( \left( xx' + \gamma k  \mathbb{I}_{k} \right)^{-1} \right) &\geq& \sum_{j=1}^{k} \frac{1}{x_j^2 + \gamma k }, \\
&=& \frac{1}{k} \sum_{j=1}^{k} \frac{1}{(x_j^2/k) + \gamma },\\
&\geq& \frac{1}{k} \sum_{j=1}^{k} \frac{1}{x_j^2 + \gamma  },\\
&\geq& \frac{1}{x_1^2 + \gamma }.
\end{eqnarray*}
% Recall that for any matrix $A$, $\textrm{tr}(A)$ equals the sum of eigenvalues of $A$. Further, the eigenvalues of $A^{-1}$ are the reciprocals of the eigenvalues of matrix $A$ for an invertible matrix. Finally if $A$ is positive definite, all the eigenvalues are strictly positive. 

% By the Gershgorin circle theorem (see e.g. Theorem 6.1.1 of \cite{horn1990matrix}), all the eigenvalues of a matrix $A$ lie within $\bigcup_{\kappa=1}^k [a_{\kappa,\kappa} - R_\kappa, a_{\kappa,\kappa} + R_\kappa ]$ where $R_\kappa$ is the sum of the absolute values of the non-diagonal terms on row $\kappa$, and $a_{\kappa,\kappa}$ is the $\kappa$ diagonal element.   

% Consider the matrix $(X'X + \gamma k \mathbb{I}_k)$.
% Observe that $R_\kappa$ in this case = $|x_\kappa|(\sum_{\kappa' \neq \kappa} |x_{\kappa'}|)$, while $a_{\kappa,\kappa} = x_\kappa^2 + k\gamma$. Therefore the largest possible eigenvalue is $|x_1| (\sum_{\kappa} |x_\kappa|) + k \gamma$, which in turn is small than $k (x_1^2 + \gamma)$. 

% Therefore for the matrix $(X'X + \gamma k \mathbb{I}_k)^{-1}$, all eigenvalues are larger than $\frac{1}{k (x_1^2 + \gamma)}$, and therefore the sum of eigenvalues is at least $\frac{1}{(x_1^2 + \gamma)}$ (since there are $k$ eigenvalues)!
We can therefore conclude that 
\begin{align*}
 \mathrm{tr}\left[\left(X'X + \gamma k \mathbb{I}_k\right)^{-1}\right] \geq \frac{1}{x_1^2 + \gamma},
\end{align*}
as desired. 

We are left to prove that:
\begin{align*}
&(1- X(X'X + \gamma k \mathbb{I}_k)^{-1}X') \geq \frac{\gamma}{x_1^2 + \gamma},\\
\iff& X(X'X + \gamma k \mathbb{I}_k)^{-1}X' \leq \frac{x_1^2}{x_1^2 + \gamma}.
\end{align*}
Now, observe that $X(X'X + \gamma k \mathbb{I}_k)^{-1}X'$ is a scalar. We know that for a scalar, $a = \text{tr}(a)$. Therefore we have that
\begin{align*}
&X(X'X + \gamma k \mathbb{I}_k)^{-1}X',\\
=& \mathrm{tr}[X(X'X + \gamma k \mathbb{I}_k)^{-1}X'],\\
=& \mathrm{tr}[(X'X + \gamma k \mathbb{I}_k)^{-1}X'X],\\
=& \mathrm{tr}[(\frac{1}{\gamma k} X'X +  \mathbb{I}_k)^{-1}\frac{1}{\gamma k}X'X].
\intertext{Denote $\frac{1}{\gamma k} X'X $ as $A$. Substituting}
=& \mathrm{tr}[(A +  \mathbb{I}_k)^{-1}A].
\end{align*}
Now, observe that if $\lambda$ is an eigenvalue of $A$, then $\frac{\lambda}{1+ \lambda}$ is an eigenvalue of $(A +  \mathbb{I}_k)^{-1}A$. To see this, suppose $v$ is an eigenvector of $A$ with eigenvalue $\lambda$. Then, 
\begin{align*}
&A v = \lambda v, \\
\implies& (A+ \mathbb{I}_k) v = (\lambda+1) v ,\\
\implies & (A+ \mathbb{I}_k)^{-1} v = \frac{1}{1+\lambda}v ,\\
\implies & (A+ \mathbb{I}_k)^{-1} A v = \frac{\lambda}{1+\lambda}v .
\end{align*}
Substituting this in, we have
\begin{align*}
\mathrm{tr}[(A +  \mathbb{I}_k)^{-1}A]=& \sum_{i=1}^k \frac{\lambda_i}{1+\lambda_i}.
\end{align*}
Therefore we are left to show that
\begin{align*}
&\sum_{i=1}^k \frac{\lambda_i}{1+\lambda_i} \leq \frac{x_1^2}{x_1^2 + \gamma}
\end{align*}
Here $\lambda_i$'s are the eigenvalues of $\frac{1}{\gamma k} X'X$. This  implies that $\sum_i \lambda_i = \frac{1}{\gamma k} \sum_i x_i^2.$

Note that $X'X$ is not full rank, indeed, its null space is of dimension $k-1$. Therefore it has $k-1$ multiplicity eigenvalue of $0$. The unique non-zero eigenvalue must then be $ \frac{1}{\gamma k} \sum_i x_i^2$. 

Substituting in, we have 
\begin{align*}
\sum_{i=1}^k \frac{\lambda_i}{1+\lambda_i}=& \frac{\frac{1}{\gamma k} \sum_i x_i^2}{\frac{1}{\gamma k} \sum_i x_i^2 + 1},\\
=& \frac{\frac{1}{k} \sum_i x_i^2}{\frac{1}{ k} \sum_i x_i^2 + \gamma},\\
\leq & \frac{x_1^2}{x_1^2 + \gamma}.
\end{align*}
where the last inequality follows since we assumed that $x_1^2 = \max_i \{x_i^2: 1 \leq i \leq k \}$.
\end{proof}

\begin{restatable}{proposition}{highprobwinner}
\label{prop:highprobwinner} 
Suppose all agents have Normal-Inverse Gamma priors with shared hyper-parameters $(a_0,b_0, \gamma)$, and believe the joint distribution of the covariates, $P$, is such that $\mathbb{E}_P[xx'] = \mathbb{I}_k$. Fix the true DGP $\mathbb{P}$ and size of dataset $n$. Consider any agent with prior $\pi$ and model $J(\pi)$. For any $p \in (0,1)$ there exists $b_0$ large enough so
\begin{align*}
    \mathbb{P}\left(D_n : \min_{\pi': J(\pi') \subset J(\pi)} L^*(\pi',D_n) < L^*(\pi, D_n) \right) >p,
\end{align*}
i.e. with probability at least $p$ over datasets $D_n$, there exists an agent with prior $\pi'$ with $J(\pi') \subset J(\pi)$, with a lower posterior expected loss, i.e. $L^*(\pi',D_n) < L^*(\pi, D_n)$.
\end{restatable}

\begin{proof}
To see this, recall again the formulas for posteriors (\ref{equation:PosteriorMeanSigma}, \ref{equation:PosterVariance}): 
\begin{align*}
&\mathbb{E}_\pi[\seps|D_n] = \frac{\frac{2b_0}{n} + \frac{1}{n}\min_{\beta \in \mathbb{R}^{|J(\pi)|}} (y-X_{J(\pi)}\beta)'(y-X_{J(\pi)}\beta) + (\gamma |J(\pi)|) \,  ||\beta||^2  }{\frac{2 a_0}{n} + 1 - \frac{2}{n} },
\\
&\mathbb{V}_{\pi}[\beta_{J(\pi)}|D_n] = \mathbb{E}_{\pi} \left[\seps | D_n\right] (X_{J(\pi)}' X_{J(\pi)} + (\gamma |J(\pi)|) \mathbb{I}_{|J(\pi)|})^{-1}.
\end{align*}

Further, by Lemma \ref{lemma:1agentposteriorloss} and the fact that $E[xx'] = \mathbb{I}_k$, we have that:
\begin{align*}
    L(\pi, D_n) &= \mathbb{E}_\pi[\seps|D_n] + \textrm{tr}(\mathbb{V}_{\pi}[\beta_{J(\pi)}|D_n]),\\
    &= \mathbb{E}_\pi[\seps|D_n] \left(1+ \textrm{tr}\left( (X_{J(\pi)}' X_{J(\pi)} + (\gamma |J(\pi)|) \mathbb{I}_{|J(\pi)|})^{-1}\right) \right).
\end{align*}
Therefore, we have that for any two priors $\pi, \pi'$:
\begin{align*}
    &L(\pi, D_n) \leq L(\pi', D_n),\\
    \iff &   \frac{\mathbb{E}_\pi[\seps|D_n]}{ \mathbb{E}_{\pi'}[\seps|D_n] } \leq \frac{1+ \textrm{tr}\left( (X_{J(\pi')}' X_{J(\pi')} + (\gamma |J(\pi')|) \mathbb{I}_{|J(\pi')|})^{-1}\right)}{1+ \textrm{tr}\left( (X_{J(\pi)}' X_{J(\pi)} + (\gamma |J(\pi)|) \mathbb{I}_{|J(\pi)|})^{-1}\right)},\\
\intertext{Note that we know that the left hand side,}
&\frac{\mathbb{E}_\pi[\seps|D_n]}{ \mathbb{E}_{\pi'}[\seps|D_n] } = \frac{2b_0 + \min_{\beta \in \mathbb{R}^|J(\pi)|} (y-X_{J(\pi)}\beta)'(y-X_{J(\pi)}\beta) + (\gamma |J(\pi)|) \,  ||\beta||^2  }{2b_0+ \min_{\beta \in \mathbb{R}^|J(\pi')|} (y-X_{J(\pi')}\beta)'(y-X_{J(\pi')}\beta) + (\gamma |J(\pi')|) \,  ||\beta||^2  }
\end{align*}
Therefore as $b_0$ grows large, we have that (the left hand side) $\frac{\mathbb{E}_\pi[\seps|D_n]}{ \mathbb{E}_{\pi'}[\seps|D_n] }  \to_P 1$. 

However, observe that the right hand side is independent of $b_0$. Further, we know, from the proof of Proposition \ref{prop:knownvariance} that there exists $\pi'$ with $J(\pi') \subset J(\pi)$ such that $$\textrm{tr}\left( (X_{J(\pi')}' X_{J(\pi')} + (\gamma |J(\pi')|) \mathbb{I}_{|J(\pi')|})^{-1}\right) < \textrm{tr}\left( (X_{J(\pi)}' X_{J(\pi)} + (\gamma |J(\pi)|) \mathbb{I}_{|J(\pi)|})^{-1} \right).$$ Further, there are only a finite number of priors $\pi'$ with $J(\pi') \subset J(\pi)$ (since all the priors share hyper-parameters by assumption,  the model uniquely determines the prior and there are only a finite collection of subsets of $J(\pi)$). Therefore, for $b_0$ large enough, with probability close to $1$ over the true distribution of $D_n$, we have that there exists $\pi'$ with the desired properties such that $L(\pi', D_n) < L(\pi, D_n)$ as desired. 
\end{proof}

\begin{proof}
To see this, recall again the formulas for posteriors (\ref{equation:PosteriorMeanSigma}, \ref{equation:PosterVariance}): 
\begin{align*}
&\mathbb{E}_\pi[\seps|D_n] = \frac{\frac{2b_0}{n} + \frac{1}{n}\min_{\beta \in \mathbb{R}^{|J(\pi)|}} (y-X_{J(\pi)}\beta)'(y-X_{J(\pi)}\beta) + (\gamma |J(\pi)|) \,  ||\beta||^2  }{\frac{2 a_0}{n} + 1 - \frac{2}{n} },
\\
&\mathbb{V}_{\pi}[\beta_{J(\pi)}|D_n] = \mathbb{E}_{\pi} \left[\seps | D_n\right] (X_{J(\pi)}' X_{J(\pi)} + (\gamma |J(\pi)|) \mathbb{I}_{|J(\pi)|})^{-1}.
\end{align*}

Further, by Lemma \ref{lemma:1agentposteriorloss} and the fact that $E[xx'] = \mathbb{I}_k$, we have that:
\begin{align*}
    L(\pi, D_n) &= \mathbb{E}_\pi[\seps|D_n] + \textrm{tr}(\mathbb{V}_{\pi}[\beta_{J(\pi)}|D_n]),\\
    &= \mathbb{E}_\pi[\seps|D_n] \left(1+ \textrm{tr}\left( (X_{J(\pi)}' X_{J(\pi)} + (\gamma |J(\pi)|) \mathbb{I}_{|J(\pi)|})^{-1}\right) \right).
\end{align*}
Therefore, we have that for any two priors $\pi, \pi'$:
\begin{align*}
    &L(\pi, D_n) \leq L(\pi', D_n),\\
    \iff &   \frac{\mathbb{E}_\pi[\seps|D_n]}{ \mathbb{E}_{\pi'}[\seps|D_n] } \leq \frac{1+ \textrm{tr}\left( (X_{J(\pi')}' X_{J(\pi')} + (\gamma |J(\pi')|) \mathbb{I}_{|J(\pi')|})^{-1}\right)}{1+ \textrm{tr}\left( (X_{J(\pi)}' X_{J(\pi)} + (\gamma |J(\pi)|) \mathbb{I}_{|J(\pi)|})^{-1}\right)},\\
\intertext{Note that we know that the left hand side,}
&\frac{\mathbb{E}_\pi[\seps|D_n]}{ \mathbb{E}_{\pi'}[\seps|D_n] } = \frac{2b_0 + \min_{\beta \in \mathbb{R}^|J(\pi)|} (y-X_{J(\pi)}\beta)'(y-X_{J(\pi)}\beta) + (\gamma |J(\pi)|) \,  ||\beta||^2  }{2b_0+ \min_{\beta \in \mathbb{R}^|J(\pi')|} (y-X_{J(\pi')}\beta)'(y-X_{J(\pi')}\beta) + (\gamma |J(\pi')|) \,  ||\beta||^2  }
\end{align*}
Therefore as $b_0$ grows large, we have that (the left hand side) $\frac{\mathbb{E}_\pi[\seps|D_n]}{ \mathbb{E}_{\pi'}[\seps|D_n] }  \to_P 1$. 

However, observe that the right hand side is independent of $b_0$. Further, we know, from the proof of Proposition \ref{prop:knownvariance} that there exists $\pi'$ with $J(\pi') \subset J(\pi)$ such that $$\textrm{tr}\left( (X_{J(\pi')}' X_{J(\pi')} + (\gamma |J(\pi')|) \mathbb{I}_{|J(\pi')|})^{-1}\right) < \textrm{tr}\left( (X_{J(\pi)}' X_{J(\pi)} + (\gamma |J(\pi)|) \mathbb{I}_{|J(\pi)|})^{-1} \right).$$ Further, there are only a finite number of priors $\pi'$ with $J(\pi') \subset J(\pi)$ (since all the priors share hyper-parameters by assumption,  the model uniquely determines the prior and there are only a finite collection of subsets of $J(\pi)$). Therefore, for $b_0$ large enough, with probability close to $1$ over the true distribution of $D_n$, we have that there exists $\pi'$ with the desired properties such that $L(\pi', D_n) < L(\pi, D_n)$ as desired. 
\end{proof}

\begin{restatable}{theorem}{winnerfixedn}
\label{prop:winner-fixed-n}
Suppose all the agents have Normal-Inverse Gamma prior with shared hyper-parameters $(a_o, b_n, \gamma)$, where $b_n \in \omega \left( n ^{2}\right)$.\footnote{Roughly, that $b_n$ asymptotically grows at a rate strictly faster than $n^2$.} Suppose the DGP $\mathbb{P}$ satisfies Assumption \ref{ass: high-level-easy}, with parameter $\theta_0 := (\beta_0, \sigma_0^2)$.  Let $J_0$ denote the associated true model for $\beta_0$ and suppose there exists at least one agent with prior $\pi$ such that $|J(\pi)| < J_0$. Then
$$\lim_{n \rightarrow \infty} \mathbb{P} \left(  \exists \pi \in \argmin_{\pi \in \Pi} L^*(\pi, D_n)  \textrm{ s.t }  |J(\pi)|<|J_0|      \right) = 1.$$
\end{restatable}

\begin{proof}
It is well known that for a prior $\pi$ in the Normal-Inverse Gamma family:
\begin{eqnarray*}
\mathbb{V}_{\pi}[\beta_{J(\pi)}|D_n] &=& \mathbb{E}_{\pi} \left[\seps | D_n\right] (X_{J(\pi)}' X_{J(\pi)} + \gamma |J(\pi)| \mathbb{I}_{|J(\pi)|})^{-1},\\
&=& \mathbb{E}_{\pi} \left[\seps | D_n\right] \frac{1}{n} \left( \frac{X_{J(\pi)}' X_{J(\pi)}}{n} + \frac{\gamma |J(\pi)| \mathbb{I}_{|J(\pi)|}}{n} \right)^{-1}.
\end{eqnarray*}
Under Assumption \ref{ass: high-level-easy},
$$ \left( \frac{X_{J(\pi)}' X_{J(\pi)}}{n} + \frac{\gamma |J(\pi)| \mathbb{I}_{|J(\pi)|}}{n} \right)^{-1} =   \mathbb{E}_{\mathbb{P}}[x_{J(\pi)}x_{J(\pi)}']^{-1} + o_{\mathbb{P}}(1).  $$    
Consequently,
\begin{equation*}
\textrm{tr}\left( \mathbb{V}_{\pi}[\beta_{J(\pi)}|D_n] \mathbb{E}_{\mathbb{P}}[x_{J(\pi)}x_{J(\pi)}'] \right) = \mathbb{E}_{\pi} \left[\seps | D_n\right] \left( \frac{J(\pi)}{n} + o_{\mathbb{P}}\left( \frac{1}{n} \right) \right).
\end{equation*}
It follows from algebra that for any priors $\pi$, $\pi'$ in the Normal-Inverse Gamma family
\begin{align*}
&L^*(\pi', D_n) > L^*(\pi,D_n)\\
\iff&\left( \mathbb{E}_{\pi} \left[\seps | D_n\right] - \mathbb{E}_{\pi'} \left[\seps | D_n\right] \right) \left( 1+ \frac{J(\pi')}{n} + o_{\mathbb{P}} \left( \frac{1}{n} \right) \right) 
>\mathbb{E}_{\pi}[\sigma^2_{\epsilon}|D_n] \left( \frac{J(\pi)-J(\pi')}{n} \right).
\end{align*}

It is well known that for a prior $\pi$ in the Normal-Inverse Gamma family, the posterior mean of $\beta_{J(\pi)}$ is the `Ridge estimator'
\[ \widehat{\beta}_{\pi} : = (X_{J(\pi)}'X_{J(\pi)} + \gamma |J(\pi)|\mathbb{I}_{J(\pi)})^{-1}X_{J(\pi)}'y,\]
which solves the problem

\[ \min_{\beta \in \mathbb{R}^{|J(\pi)|}} (y-X_{J(\pi)}\beta)'(y-X_{J(\pi)}\beta) + (\gamma |J(\pi)|) \,  ||\beta||^2  \]

\noindent First, consider two priors $\pi,\pi'$ such that $J(\pi') \subset J(\pi)$, and $J(\pi') = J_0$. In a slight abuse of notation let $\widehat{\beta}_{\pi'}$ denote the vector in $\mathbb{R}^{|J(\pi)|}$ with all the coordinates in $J(\pi) \backslash J(\pi')$ equal to zero. Also, let $J$ be used to abbreviate  $J(\pi)$.

\noindent Equation \eqref{equation:PosteriorMeanSigma} implies that for any such two priors $\pi,\pi'$
\[n(\mathbb{E}_{\pi'}[\seps|D_n] -\mathbb{E}_{\pi}[\seps|D_n]) \]

\noindent is proportional to the sum of

\begin{equation}\label{equation:aux1}
  (y-X_J\widehat{\beta}_{\pi'})'(y-X_J \widehat{\beta}_{\pi'}) - (y-X_J\widehat{\beta}_{\pi})'(y-X_J \widehat{\beta}_{\pi})
\end{equation}
and
\begin{equation}\label{equation:aux2}
\gamma \left( |J(\pi')| \,  ||\widehat{\beta}_{\pi'}||^2  -  
 |J| \,  ||\widehat{\beta}_{\pi}||^2  \right).
\end{equation}
\noindent where the proportionality constant is $c_n := (2 a_0/n + 1 - 2/n)^{-1}$.

\noindent Algebra shows that the expression in \eqref{equation:aux1} equals
\[ -2(y-X_{J}\widehat{\beta}_{\pi})'X_{J} (\widehat{\beta}_{\pi'}-\widehat{\beta}_{\pi}) + (\widehat{\beta}_{\pi}-\widehat{\beta}_{\pi'})'X'_JX_J (\widehat{\beta}_{\pi}-\widehat{\beta}_{\pi'})  \]
and the expression in \eqref{equation:aux2} 
\[ \gamma |J(\pi')|(\widehat{\beta}_{\pi}-\widehat{\beta}_{\pi'})'(\widehat{\beta}_{\pi}-\widehat{\beta}_{\pi'}) - \gamma (|J|-|J(\pi')|) \widehat{\beta}'_{\pi}\widehat{\beta}_{\pi} + 2\gamma |J(\pi')| \widehat{\beta}'_{\pi}(\widehat{\beta}_{\pi'}-\widehat{\beta}_{\pi}).    \]

\noindent The first-order conditions defining the Ridge estimator imply
\[-2(y-X_{J}\widehat{\beta}_{\pi})'X_{J} + 2\gamma |J| \widehat{\beta}'_{\pi} = 0. \]
Therefore, in any finite sample
\begin{align*}
n(\mathbb{E}_{\pi'}[\seps|D_n] -\mathbb{E}_{\pi}[\seps|D_n]) =& c_n \big ( (\widehat{\beta}_{\pi}-\widehat{\beta}_{\pi'})'(X'_JX_J+ \gamma|J(\pi')| \mathbb{I}_{J} ) (\widehat{\beta}_{\pi}-\widehat{\beta}_{\pi'}) \\
&+ \gamma (|J|-|J(\pi')|) \widehat{\beta}'_{\pi}\widehat{\beta}_{\pi} - 2 \gamma (|J|-|J(\pi')|) \widehat{\beta}'_{\pi'}\widehat{\beta}_{\pi} \big ).
\intertext{Under Assumption \ref{ass: high-level-easy} and recalling that $J(\pi') = J_0$,}
=& O_{\mathbb{P}}(1).
\end{align*}
However, under the same assumption
\[ \mathbb{E}_{\pi}[\seps|D_n] = \frac{2 b_n}{n} + O_{\mathbb{P}}(1).  \]
Since $b_n \in \omega \left( n^{2} \right)$, the previous term diverges to infinity. This implies
\[\mathbb{P} \left( n(\mathbb{E}_{\pi'}[\seps|D_n] -\mathbb{E}_{\pi}[\seps|D_n]) \left(1+ \frac{J(\pi')}{n} + o_{\mathbb{P}}(1) \right) > \mathbb{E}_{\pi}[\seps|D_n]) (J(\pi)-J(\pi'))  \right) \]
converges to zero. We conclude that $J(\pi) \supset J(\pi') =J_0$ implies 
$$\mathbb{P}[ L^*(\pi,D_n) < L^*(\pi', D_n) ]  \rightarrow 0.$$

Now instead consider the same framework as above, but let $\pi$ now be such that $J(\pi) = J_0$ and $|J(\pi')| < |J(\pi)]$. The probability that the smaller model, $\pi'$, is defeated by $\pi$ is
\[\mathbb{P} \left( (\mathbb{E}_{\pi'}[\seps|D_n] -\mathbb{E}_{\pi}[\seps|D_n]) \left(1+ \frac{J(\pi')}{n} + o_{\mathbb{P}}(1) \right) > \frac{\mathbb{E}_{\pi}[\seps|D_n])}{n} (J(\pi)-J(\pi'))  \right). \]
Under the assumptions of the theorem 
\[(\mathbb{E}_{\pi'}[\seps|D_n] -\mathbb{E}_{\pi}[\seps|D_n]) = O_{\mathbb{P}}(1). \]
However, 
\[ \frac{\mathbb{E}_{\pi}[\seps|D_n])}{n} = \frac{b_n}{n^2} + o_{\mathbb{P}} \left( \frac{1}{n} \right). \]
Since $b_n \in \omega\left( n^{2} \right),$ the latter diverges as $n$ grows large. We conclude that:
$$\mathbb{P}[  L^*(\pi',D_n) < L^*(\pi,D_n) ]  \rightarrow 1.$$
The result follows. 
\end{proof}
